# Supplementary material for: Modularity through Attention: Efficient Training and Transfer of Language-Conditioned Policies for Robot Manipulation
Source: arXiv:2212.04573 source file (2022-12-08)
Supplement: Supplementary file 1 [file 01-dataset.tex]

% \section{Data Collection}
% A simulated dataset was collected for all 3 robots involved in the experiments (Kinova, UR5 and Franka). We recorded 2000 demonstrations for training a policy from scratch, and 400 for transfering a policy to an unseen robot. For each of the demonstrations, we recorded all object positions, robot proprioception (joint angle data), camera images, and end-effector positions throughout the whole trajectory at 125 Hz. As shown in Fig.~\ref{fig:super_attn_label}, we perform a transformation of the positions into image patches, thereby locating the end-effector and objects in the image. Images are collected at a resolution of 224$\times$224 resolution. Each demonstration typically comprises 100-400 timesteps. 

% For real-robot experiments, we also recorded robot proprioception, camera images and end-effector positions. A higher cost comes from collecting 3D object positions. 
% %In order to that, when objects are placed on the table, we use some tracking techniques to track the positions. Alternatively, it is also a feasible method to mark coordinate locators on the table, and thus we know the object XY position. Z position can just be marked as the object centerpoint height. After the the object is captured by the gripper, we just approximated the object position by the gripper position, so that we can avoid tracking issues caused by occlusions. We collected 340 demonstrations on a real-world UR5 robot. 
% In order to generate an estimate of the object's position, we use the robot end-effector's position after it touches the object. For higher accuracy, an object tracking algorithm can also be used instead. 

% \begin{figure}[t!]
%     \centering
%     \includegraphics[width=\linewidth]{images/sup_attn_2.pdf}
%     \caption{In order to collect labels for supervised attention in images, we firstly track the 3D position of the object, which is then projected onto the 2D image, and falls into one of the image patches. In the real world experiment, this patch along with the adjacent patches are selected as the labels.}
%     \label{fig:super_attn_label}
% \end{figure}





% % \setcounter{magicrownumbers}{0}
% \begin{table}[!t]
% \small
% \parbox{.50\linewidth}{
% % \scriptsize
% \centering
% \setlength{\tabcolsep}{0.6em}%
% % >{\columncolor[gray]{0.925}}c %
% \begin{tabular}{@{\makebox[0.8em][r]{\space}} @{\extracolsep{\fill}} c H c}
% \toprule
% \multicolumn{1}{c}{\textbf{Object}} & \multicolumn{1}{H}{\textbf{Adj}} & \multicolumn{1}{c}{\textbf{Noun}}  \\ \midrule
% % \multicolumn{1}{c}{\textbf{Model}} & \multicolumn{1}{H}{Train} & \multicolumn{1}{H}{Transf.} & Pick & Push & All & \multicolumn{1}{H}{Coke} & \multicolumn{1}{H}{Pepsi} & \multicolumn{1}{H}{Bottle} & \multicolumn{1}{H}{Cube} & \multicolumn{1}{H}{Carton} & \multicolumn{1}{H}{Bread} & TarPos & TrjErr & JntErr \\ \midrule
% \multirow{3}{*}{Coke}  & red       & can \\
%                       & coke      & bottle \\
%                       & cocacola  & \\ \midrule
% \multirow{3}{*}{Pepsi} & blue       & can \\
%                       & pepsi      & bottle \\
%                       & pepsi coke & \\\midrule
% \multirow{4}{*}{Bottle} & green      & bottle \\
%                         & glass      & \\
%                         & `'         & \\
%                         & green glass& \\\midrule
% \multirow{2}{*}{Carton} & milk       & carton \\
%                         & white      & box \\ \midrule
% \multirow{3}{*}{Cube}   & red        & object \\
%                         & maroon     & cube \\
%                         &    & square \\ \midrule
% \multirow{3}{*}{Bread}  & `'         & bread \\
%                         &            & yellow object \\
%                         &      & brown object \\
% \bottomrule

% \end{tabular}
% \caption{The noun phrase template.}
%  \label{tab:noun-template}

% \vspace{0.2in}
% % \scriptsize
% \centering
% \setlength{\tabcolsep}{0.6em}%
% % >{\columncolor[gray]{0.925}}c %
% \begin{tabular}{@{\makebox[0.6em][r]{\space}} @{\extracolsep{\fill}} c H c}
% \toprule
% \multicolumn{1}{c}{\textbf{Verb Pick}} & \multicolumn{1}{H}{\textbf{Verb Push}} & \multicolumn{1}{c}{\textbf{Verb Put}} \\ \midrule
% % \multicolumn{1}{c}{\textbf{Model}} & \multicolumn{1}{H}{Train} & \multicolumn{1}{H}{Transf.} & Pick & Push & All & \multicolumn{1}{H}{Coke} & \multicolumn{1}{H}{Pepsi} & \multicolumn{1}{H}{Bottle} & \multicolumn{1}{H}{Cube} & \multicolumn{1}{H}{Carton} & \multicolumn{1}{H}{Bread} & TarPos & TrjErr & JntErr \\ \midrule
%                     pick     & push & put down \\
%                     pick up  & move & place down \\
%                     raise  &  &\\
% \bottomrule

% \end{tabular}
% \caption{The verb phrase template.}
%  \label{tab:verb-template}
%  }
% \parbox{.45\linewidth}{

% \centering
% \setlength{\tabcolsep}{0.6em}%
% % >{\columncolor[gray]{0.925}}c %
% \begin{tabular}{@{\makebox[1em][r]{\space}} @{\extracolsep{\fill}} lH}
% \toprule
% \multicolumn{1}{c}{\textbf{Annotator Labeled Sentences}} & \multicolumn{1}{H}{\textbf{Success}} \\ \midrule
% Grab the loafs & F \\
% put down the sierra mist F lime soda & T \\
% lay down the red block & T \\
% tip over the azure can & T \\
% lift the white carton & F \\
% knock over the pastry pastry & T \\
% lift the coke can & T \\
% put down the sprite & T \\
% grab the pepsi & T \\
% elevate the red cube & T \\
% Pick up the red cube & T \\
% Lift up the blue cylinder & T \\
% Move away the brown object & T \\
% Push away the white object & T \\
% Lift the blue object & T \\
% Put down the green sprite & T \\
% Push the green sprite & T \\
% Push the reddish can & T \\
% Pick up the milk container & F \\
% Hold up the milk carton & F \\
% Please pick up the green thing. & F \\
% Lift the red colored coke can. & T \\
% Push the yellow bread. & T \\
% Grab the blue colored can. & T \\
% Nudge that green bottle. & F \\
% Put down the red colored cuboid. & T \\
% Lift the white box. & T \\
% Take the pepsi off the table. & F \\
% Push the green object forward. & F \\
% Put down the zero coke on the desk & T \\
% \bottomrule

% \end{tabular}
% \caption{Sentences collected from annotators.}
%  \label{tab:sentences-annotators}
% }
% \end{table}

% For learning natural language instructions,  we use a template to generate well-formed sentences during demonstrations. The template first randomly chooses a verb phrase according to Tab.~\ref{tab:verb-template}, and then determines a noun phrase by randomly picking from Adj and Noun in Tab.~\ref{tab:noun-template}. We leverage this procedure to generate sentences during training, validating and testing. In addition, we also collected 30 natural language sentences from human annotators. The full list can be found in Tab.~\ref{tab:sentences-annotators}. 



% % % \setcounter{magicrownumbers}{0}
% % \begin{table}[]
% % % \scriptsize
% % \centering
% % \setlength{\tabcolsep}{0.8em}%
% % % >{\columncolor[gray]{0.925}}c %
% % \begin{tabular}{@{\makebox[1em][r]{\space}} @{\extracolsep{\fill}} c H c}
% % \toprule
% % \multicolumn{1}{c}{\textbf{Object}} & \multicolumn{1}{H}{\textbf{Adj}} & \multicolumn{1}{c}{\textbf{Noun}}  \\ \midrule
% % % \multicolumn{1}{c}{\textbf{Model}} & \multicolumn{1}{H}{Train} & \multicolumn{1}{H}{Transf.} & Pick & Push & All & \multicolumn{1}{H}{Coke} & \multicolumn{1}{H}{Pepsi} & \multicolumn{1}{H}{Bottle} & \multicolumn{1}{H}{Cube} & \multicolumn{1}{H}{Carton} & \multicolumn{1}{H}{Bread} & TarPos & TrjErr & JntErr \\ \midrule
% % \multirow{3}{*}{Coke}  & red       & can \\
% %                       & coke      & bottle \\
% %                       & cocacola  & \\ \midrule
% % \multirow{3}{*}{Pepsi} & blue       & can \\
% %                       & pepsi      & bottle \\
% %                       & pepsi coke & \\\midrule
% % \multirow{4}{*}{Bottle} & green      & bottle \\
% %                         & glass      & \\
% %                         & `'         & \\
% %                         & green glass& \\\midrule
% % \multirow{2}{*}{Carton} & milk       & carton \\
% %                         & white      & box \\ \midrule
% % \multirow{3}{*}{Cube}   & red        & object \\
% %                         & maroon     & cube \\
% %                         &    & square \\ \midrule
% % \multirow{3}{*}{Bread}  & `'         & bread \\
% %                         &            & yellow object \\
% %                         &      & brown object \\
% % \bottomrule

% % \end{tabular}
% % \caption{The noun phrase template.}
% %  \label{tab:noun-template}
% % \end{table}

% % % \setcounter{magicrownumbers}{0}
% % \begin{table}[]
% % % \scriptsize
% % \centering
% % \setlength{\tabcolsep}{0.8em}%
% % % >{\columncolor[gray]{0.925}}c %
% % \begin{tabular}{@{\makebox[1em][r]{\space}} @{\extracolsep{\fill}} lc}
% % \toprule
% % \multicolumn{1}{c}{\textbf{Sentences Collected from Annotators}} & \multicolumn{1}{c}{\textbf{Success}} \\ \midrule
% % Grab the loafs & F \\
% % put down the sierra mist F lime soda & T \\
% % lay down the red block & T \\
% % tip over the azure can & T \\
% % lift the white carton & F \\
% % knock over the pastry pastry & T \\
% % lift the coke can & T \\
% % put down the sprite & T \\
% % grab the pepsi & T \\
% % elevate the red cube & T \\
% % Pick up the red cube & T \\
% % Lift up the blue cylinder & T \\
% % Move away the brown object & T \\
% % Push away the white object & T \\
% % Lift the blue object & T \\
% % Put down the green sprite & T \\
% % Push the green sprite & T \\
% % Push the reddish can & T \\
% % Pick up the milk container & F \\
% % Hold up the milk carton & F \\
% % Please pick up the green thing. & F \\
% % Lift the red colored coke can. & T \\
% % Push the yellow bread. & T \\
% % Grab the blue colored can. & T \\
% % Nudge that green bottle. & F \\
% % Put down the red colored cuboid. & T \\
% % Lift the white box. & T \\
% % Take the pepsi off the table. & F \\
% % Push the green object forward. & F \\
% % Put down the zero coke on the desk & T \\
% % \bottomrule

% % \end{tabular}
% % \caption{Sentences collected from annotators.}
% %  \label{tab:sentences-annotators}
% % \end{table}







% % % \setcounter{magicrownumbers}{0}
% % \begin{table}[]
% % % \scriptsize
% % \centering
% % \setlength{\tabcolsep}{0.8em}%
% % % >{\columncolor[gray]{0.925}}c %
% % \begin{tabular}{@{\makebox[1em][r]{\space}} @{\extracolsep{\fill}} H c H}
% % \toprule
% % \multicolumn{1}{H}{\textbf{Verb Pick}} & \multicolumn{1}{c}{\textbf{Verb Push}} & \multicolumn{1}{H}{\textbf{Verb Put Down}} \\ \midrule
% % % \multicolumn{1}{c}{\textbf{Model}} & \multicolumn{1}{H}{Train} & \multicolumn{1}{H}{Transf.} & Pick & Push & All & \multicolumn{1}{H}{Coke} & \multicolumn{1}{H}{Pepsi} & \multicolumn{1}{H}{Bottle} & \multicolumn{1}{H}{Cube} & \multicolumn{1}{H}{Carton} & \multicolumn{1}{H}{Bread} & TarPos & TrjErr & JntErr \\ \midrule
% %                     pick     & push & put down \\
% %                     pick up  & move & place down \\
% %                     raise  &  &\\
% % \bottomrule

% % \end{tabular}
% % \caption{The sentence template.}
% %  \label{tab:sentence-template}
% % \end{table}
