# Supplementary material for: Modularity through Attention: Efficient Training and Transfer of Language-Conditioned Policies for Robot Manipulation
Source: arXiv:2212.04573 source file (2022-12-08)
Supplement: Supplementary file 2 [file 03-results.tex]

\begin{figure}[t!]
    \centering
    \includegraphics[width=\linewidth]{images/exec.pdf}
    \caption{More results from tests on the simulation.}
    \label{fig:exec}
\end{figure}

\section{More Results}
In this section, we provide some more results of the transfer experiments on the simulator. Shown in Tab.~\ref{fig:exec} are executions of instructions from Kinova, UR5 and Franks robots separately. Also, our method is able to query sub-modules on the real time. Fig.~\ref{fig:aux} marks the real time prediction of end-effector position (red square) and target object position (blue circle).

\begin{figure}[t!]
    \centering
    \includegraphics[width=\linewidth]{images/aux.pdf}
    \caption{Our model can query sub-modules in the run time. Shown in the image are the end-effector position (red square) and target object position (blue circle) predictions when testing on the simulator.}
    \label{fig:aux}
\end{figure}
